# Supplementary material for: ThetA -- fast and robust clustering via a distance parameter
Source: arXiv:2102.07028 ancillary file (2021-03-01)
Supplement: Supplementary file 1 [file ThetA_Supplement.pdf]

---

## Supplement: ThetA - fast and robust clustering via a distance parameter

---

Eleftherios Garyfallidis<sup>1</sup> Shreyas Fadnavis<sup>1</sup> Jong Sung Park<sup>1</sup> Bramsh Qamar Chandio<sup>1</sup> Javier Guaje<sup>1</sup>  
Serge Koudoro<sup>1</sup> Nasim Anousheh<sup>1</sup>

To supplement the experiments explained in the main document, we conducted additional ones using the same computing environment. The following text and the mentioned figures delineate the comparisons done.

In Fig. S2 and Fig. S3, we repeat the experiment for the easy and hard cases with different number of points per cluster. The experiment was conducted in a fashion similar to the one explained in the main text. The data points were generated on a grid by randomly sampling the points from a normal distribution. The number of points per cluster was sampled from a uniform distribution in the range 10 to 50 points per cluster. This data was clustered and compared against other algorithms such as K-Means, K-Means++, BIRCH and Mini-Batch K-Means.

We show how TDG still performs better compared to other methods when the number of points per cluster are different. Fig. S4 is the result of an experiment using the same environment in Sec. 5.3 and randomly selecting the number of points per cluster from a uniform distribution. It can be seen that TDG performs well regardless of increasing the number of clusters and number of dimensions.

Fig. S5, Fig. S6 and Fig. S7 show experimental comparisons on different dimension for the experiment in Sec. 5.3. Each figure shows:  $\theta$ -sparse case where we fix the number of clusters and change the number of dimensions,  $\theta$ -sparse and  $\theta$ -dense cases where we fix the number of dimensions and change the number of clusters.

In Fig. S8 we compare TNC with other non-linear data clustering methods: Spectral Clustering, DBSCAN, Agglomerative Clustering, and OPTICS. Fig. S8-A shows that TNC merges multiple clusters into one as the number of iterations increase and until convergence. Fig. S8-B shows results on popular datasets used to benchmark non-linear clustering methods; three spirals, aggregation, compound, and two nested circles data.(Zahn, 1971) (Chang & Yeung, 2008) (Gionis et al., 2007). It can be seen that TNC yields a better clustering on all datasets, except the compound dataset with two circle like distributions. Note that TNC currently has not been optimized for speed, so the run time in the figure is not the best representative of its performance.

### References

- Chang, H. and Yeung, D.-Y. Robust path-based spectral clustering. *Pattern Recognition*, 41(1):191–203, 2008.
- Gionis, A., Mannila, H., and Tsaparas, P. Clustering aggregation. *Acm transactions on knowledge discovery from data (tkdd)*, 1(1):4–es, 2007.
- Zahn, C. T. Graph-theoretical methods for detecting and describing gestalt clusters. *IEEE Transactions on computers*, 100(1):68–86, 1971.

---

<sup>1</sup>Intelligent Systems Engineering, Indiana University Bloomington

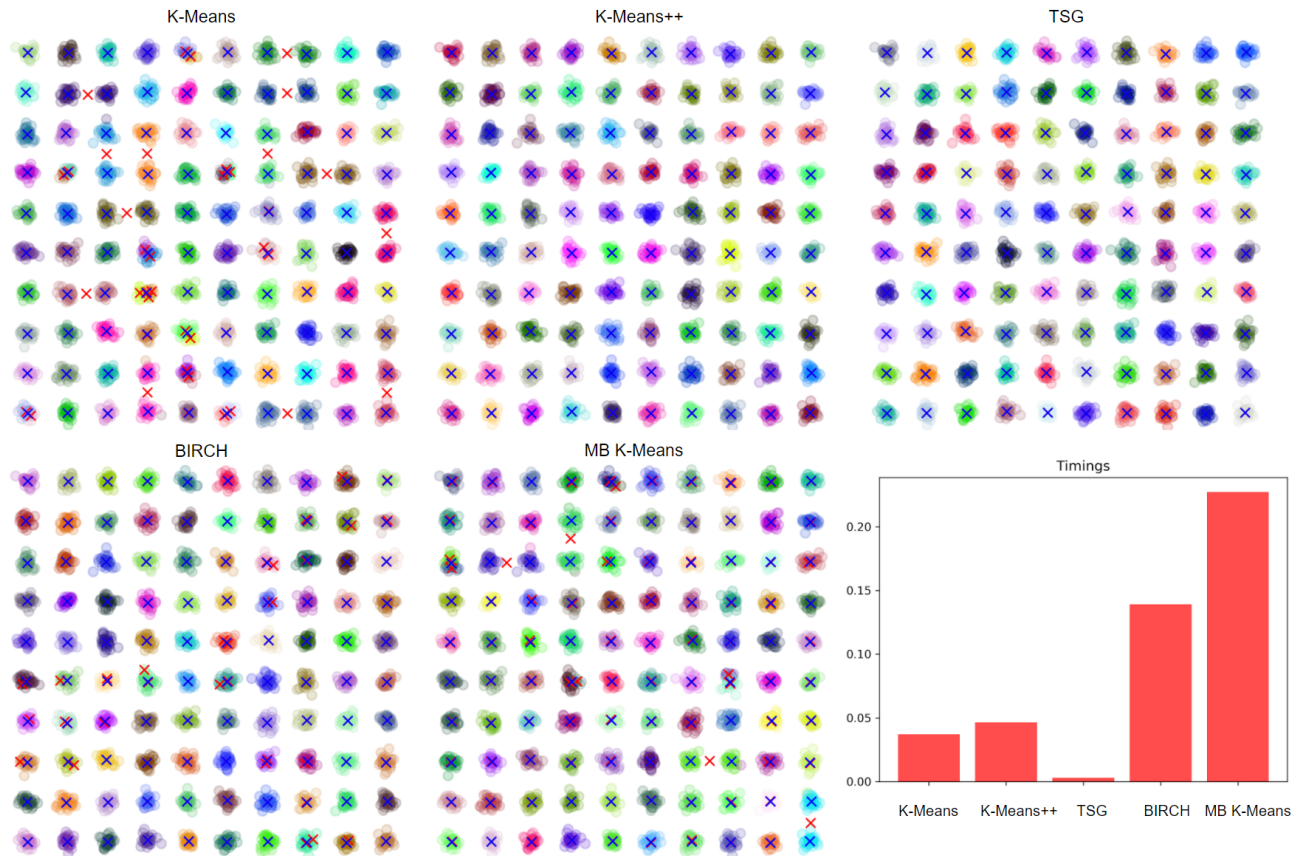

Figure S1.  $\theta$ -sparse example of 2d blobs dataset with the same number of samples per cluster, as described in Sec. 5.1.

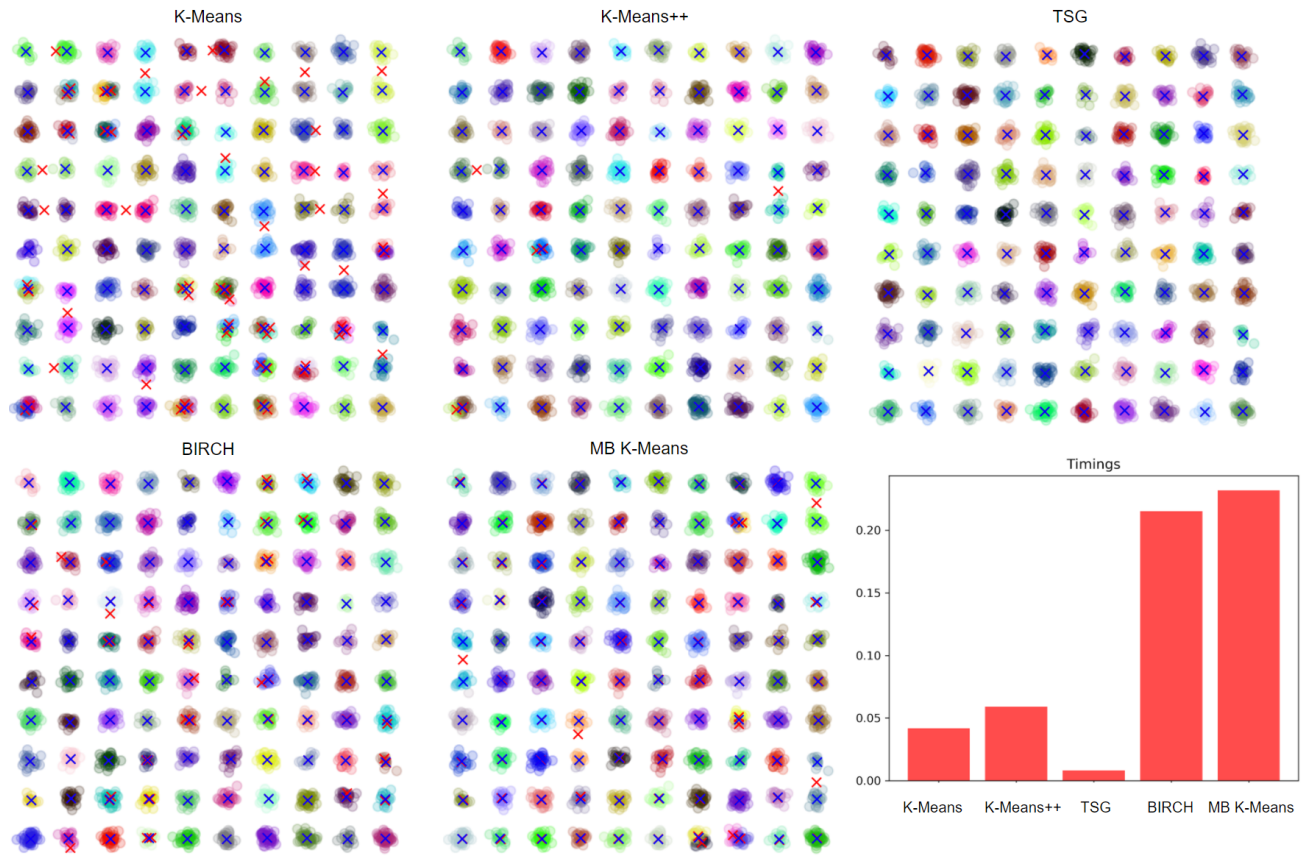

Figure S2.  $\theta$ -sparse example of 2d blobs dataset with different number of samples (randomly chosen within range 10 to 50) per cluster.

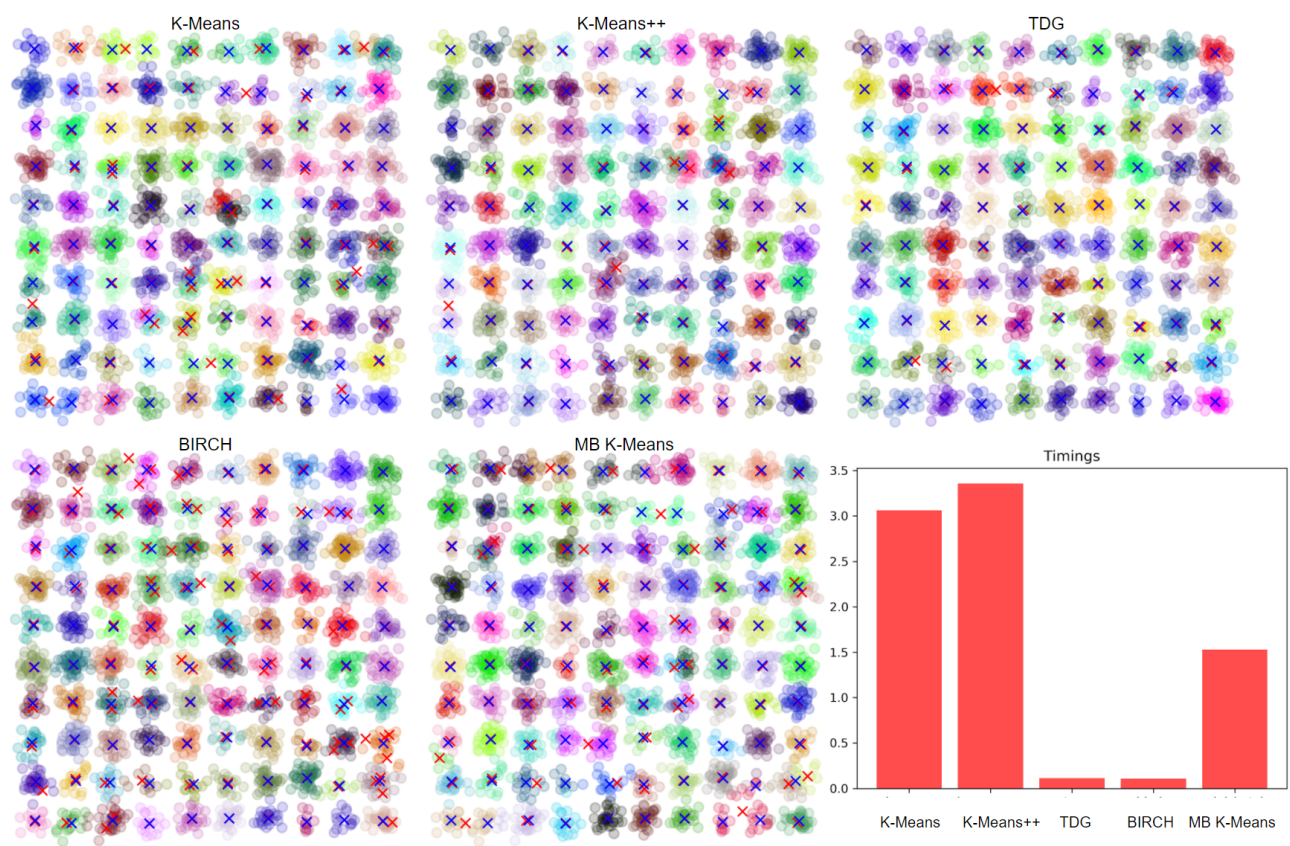

Figure S3.  $\theta$ -dense example of 2d blobs dataset with different number of samples (randomly chosen within range 10 to 50) per cluster.

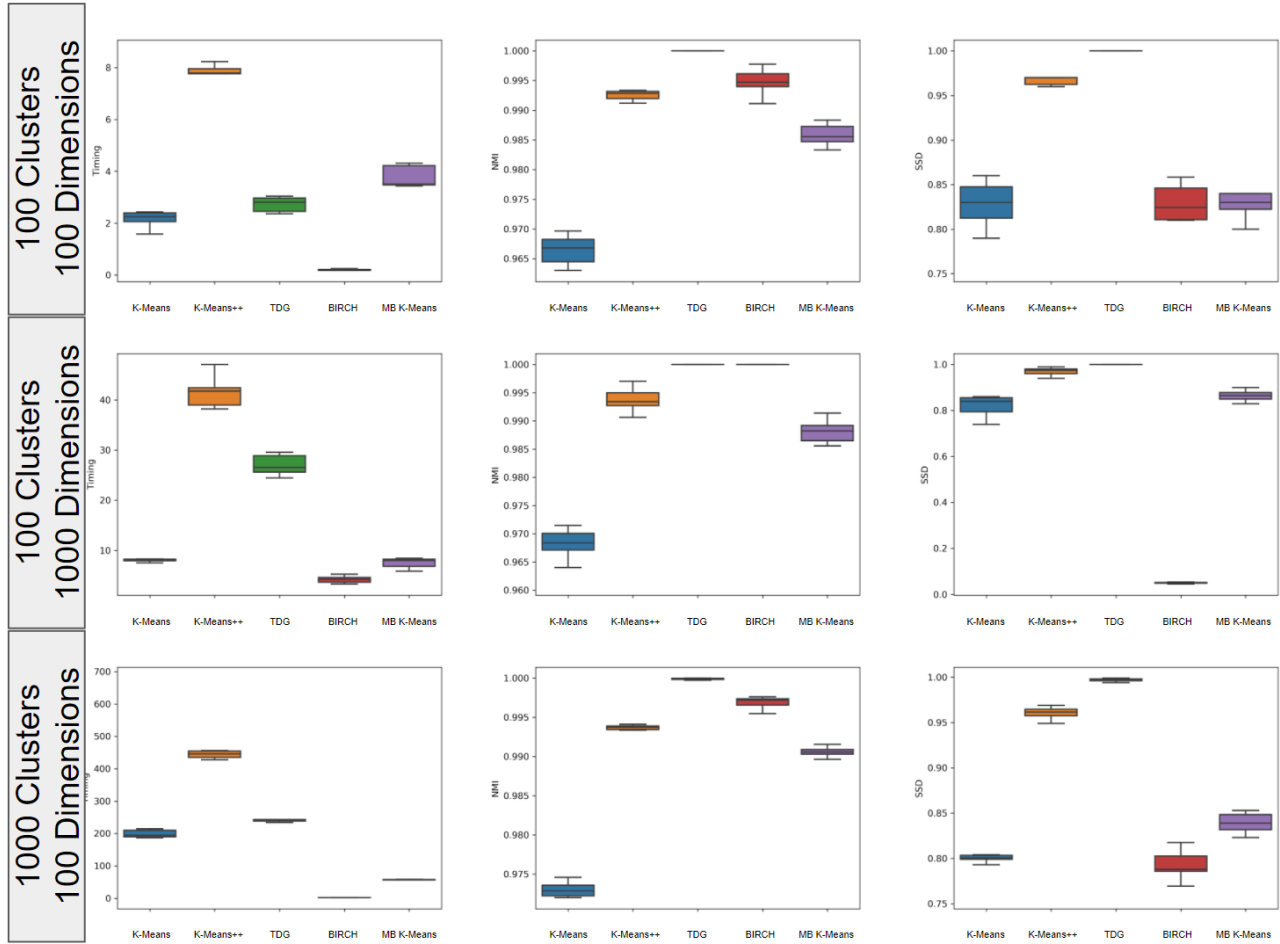

Figure S4.  $\theta$ -dense example with different number of samples (randomly chosen within range 10 to 50) per cluster. Each row corresponds to the timing (in seconds) Normalized Mutual Information (NMI) and Sum of Squared Differences (SSD) of three cases; 100 number of dimensions and 100 number of clusters, 1000 number of dimensions and 100 number of clusters, 100 number of dimensions and 1000 number of clusters

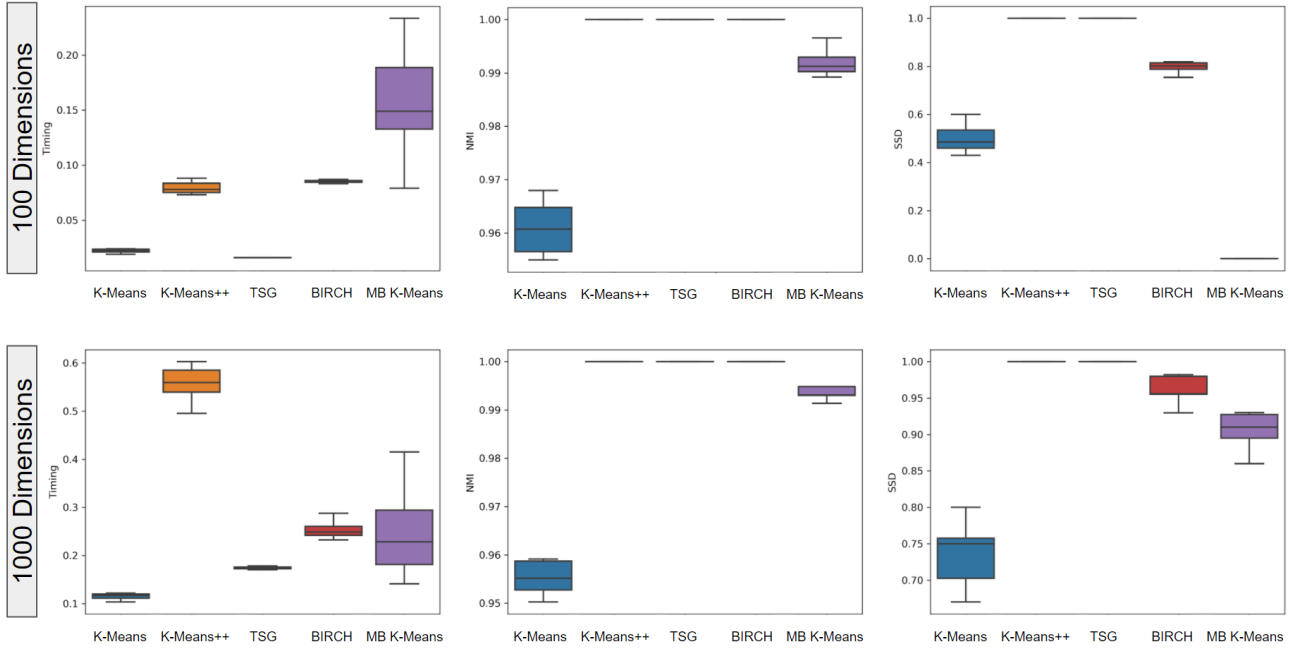

Figure S5.  $\theta$ -sparse example with 100 number of clusters with 100 dimensions(first row) and 1000 dimensions(second row). Each row shows box plots for timing(in seconds) Normalized Mutual Information(NMI) and Sum of Squared Differences metric(SSD) for each case.

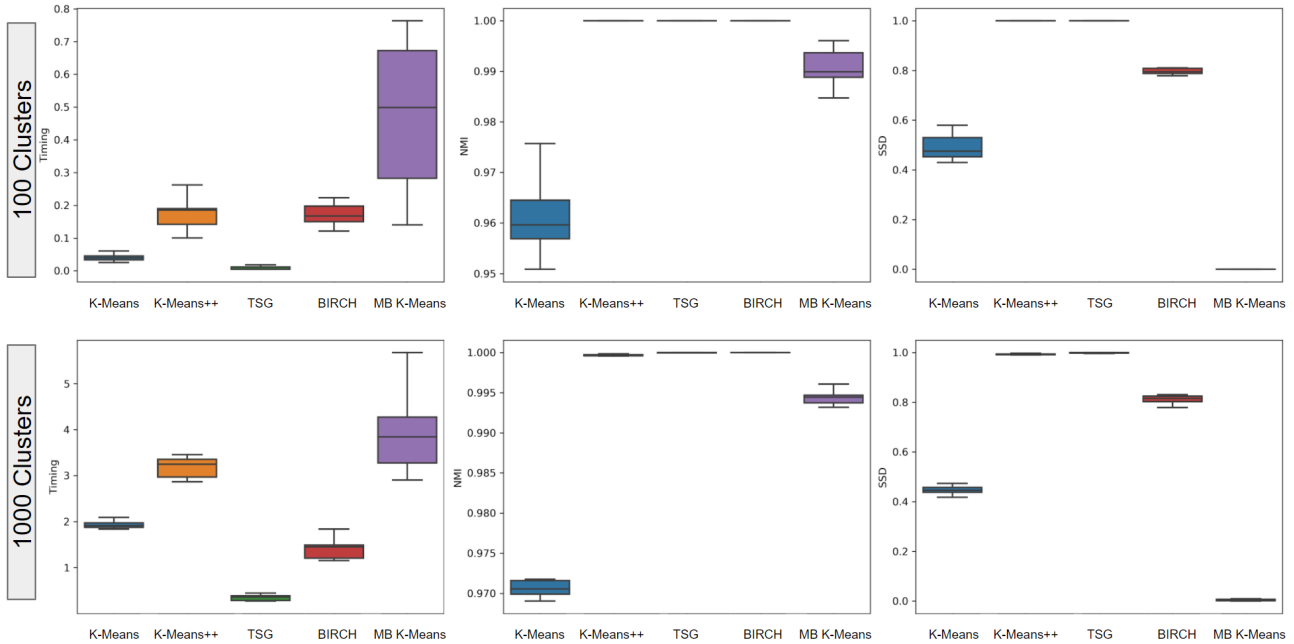

Figure S6.  $\theta$ -sparse example with 100 number of dimensions with 100 clusters(first row) and 1000 clusters(second row). Each row shows box plots for timing(in seconds) Normalized Mutual Information(NMI) and Sum of Squared Differences metric(SSD) for each case.

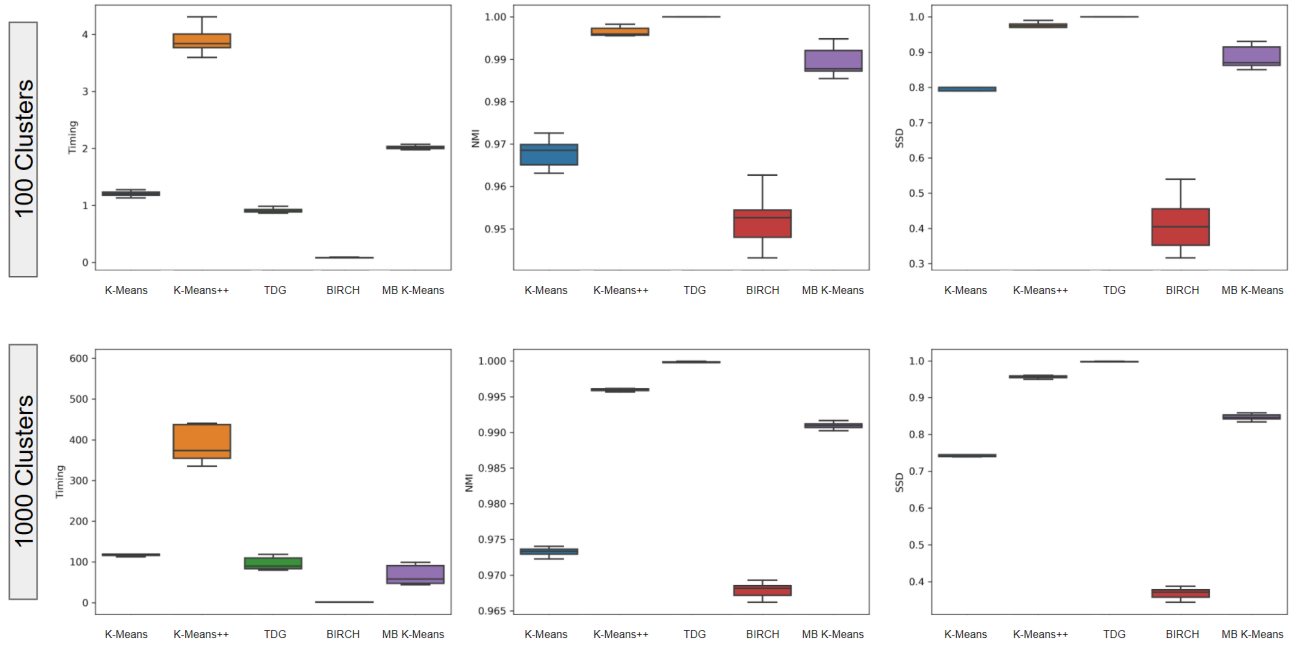

Figure S7.  $\theta$ -dense example with 100 number of dimensions with 100 clusters(first row) and 1000 clusters(second row). Each row shows box plots for timing(in seconds) Normalized Mutual Information(NMI) and Sum of Squared Differences metric(SSD) for each case.

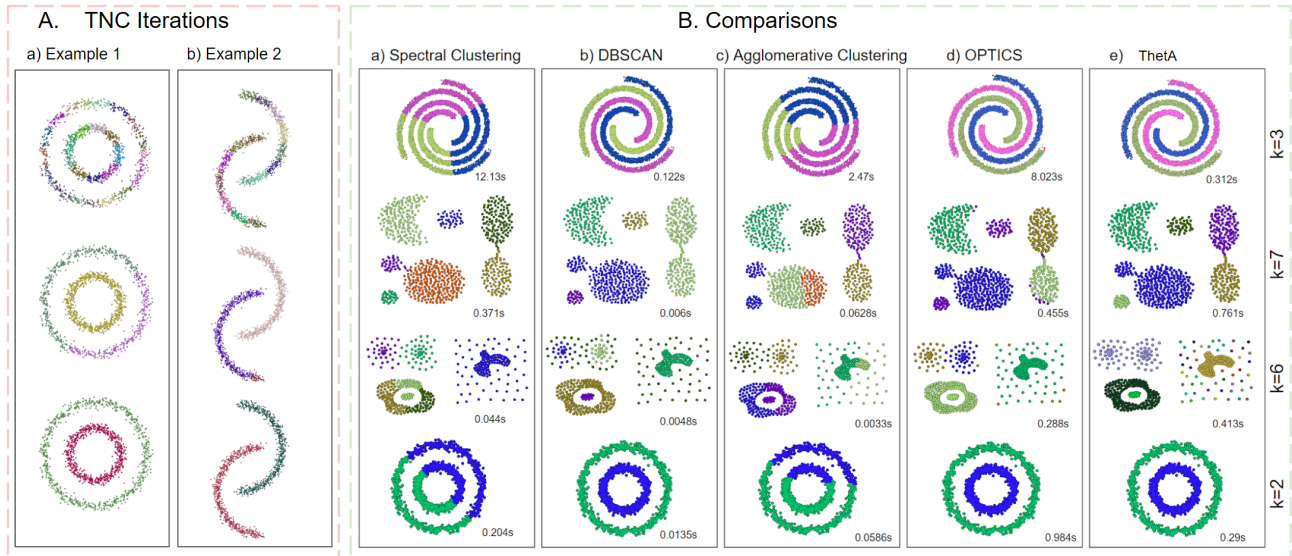

Figure S8. In the figure, part A. shows the visual explanation of how Theta Non-linear Chaining(TNC) iterations work on two examples. TNC converges to final clusters within two iterations. Part B. shows a comparison of e) TNC with famous non-linear clustering algorithms (a-d) on four different datasets. On the y-axis of the figure we have the original number of clusters in the datasets. Here, each color represents a different cluster given by clustering algorithms. Time in seconds is reported for each algorithm-dataset in the figure.
